# Supplementary material for: DocLLM: A layout-aware generative language model for multimodal document understanding
Source: arXiv:2401.00908 source file (2023-12-31)
Supplement: Supplementary file 1 [file sec_appendices.tex]

\appendix
\section{Prompting}
the template we used is as follows:

f"""Based on the given Document, {question}

Please provide only the answer (no decorations or explanations). Extract from the document when possible.

Use the following format to answer:
Answer:<answer>

Document:```{doc}```
"""

\section{Other training details}
We employed 8 AWS-based A10g GPUs, each equipped with 24GB of memory, for the pre-training process. The pre-training model is configured to run for a maximum of 5 epochs. Details of the model layer split are in Table \ref{tb:gpu_split_situ}, and GPU memory usage are provided in Table \ref{gpu_processes}.

\begin{table}[]
\centering
\caption{\label{tb:gpu_split_situ}7B model split situation}
\begin{tabular}{|c|c|}
\hline
GPU & Modules \\
\hline
0 & model.embed\_tokens, model.spatial\_embeddings, model.position\_embeddings \\
1 & Layer 0, Layer 1, Layer 2, Layer 3 \\
2 & Layer 4, Layer 5, Layer 6, Layer 7 \\
3 & Layer 8, Layer 9, Layer 10, Layer 11, Layer 12 \\
4 & Layer 13, Layer 14, Layer 15, Layer 16, Layer 17 \\
5 & Layer 18, Layer 19, Layer 20, Layer 21, Layer 22 \\
6 & Layer 23, Layer 24, Layer 25, Layer 26, Layer 27 \\
7 & Layer 28, Layer 29, Layer 30, Layer 31, norm, lm\_head \\
\hline
\end{tabular}
\end{table}

\begin{table}[h]
    \centering
    \caption{\label{tab:gpu_processes}GPU Processes Information}
    \begin{tabular}{|c|c|c|c|c|c|c|c|}
        \hline
        \textbf{GPU} & \textbf{GI} & \textbf{CI} & \textbf{PID} & \textbf{Type} & \textbf{Process name} & \textbf{GPU Memory Usage} \\
        \hline
        0 & N/A & N/A & 72863 & C & python & 5250MiB \\
        1 & N/A & N/A & 72863 & C & python & 14358MiB \\
        2 & N/A & N/A & 72863 & C & python & 21740MiB \\
        3 & N/A & N/A & 72863 & C & python & 21740MiB \\
        4 & N/A & N/A & 72863 & C & python & 21740MiB \\
        5 & N/A & N/A & 72863 & C & python & 21740MiB \\
        6 & N/A & N/A & 72863 & C & python & 21740MiB \\
        7 & N/A & N/A & 72863 & C & python & 20136MiB \\
        \hline
    \end{tabular}
\end{table}
